# Supplementary material for: Resonant interlayer coupling in NbSe$_2$-graphite epitaxial moir{\'e} superlattices
Source: arXiv:2506.00449 source file (2025-05-31)
Supplement: Supplementary file 1 [file supp.pdf]

# Supplementary Information: Resonant interlayer coupling in $NbSe_2$-graphite epitaxial moiré superlattices

S. Mo,[1,*] K. Kovalenka,[2,*] S. Buchberger,[1,3] B.K. Saika,[1] A. Azhar,[2,4] A. Rajan,[1] A. Zivanovic,[1] Y.-C. Yao,[1,3] R.V. Belosludov,[5] M.D. Watson,[6] M.S. Bahramy,[2,†] and P.D.C. King[1,‡]

[1]*SUPA, School of Physics and Astronomy, University of St Andrews, St Andrews KY16 9SS, United Kingdom*

[2]*Department of Physics and Astronomy, University of Manchester, Manchester M13 9PL, United Kingdom*

[3]*Max Planck Institute for Chemical Physics of Solids, Nöthnitzer Strasse 40, Dresden 01187, Germany*

[4]*Physics Study Program, Faculty of Science and Technology, Syarif Hidayatullah State Islamic University Jakarta, Tangerang Selatan 15412, Indonesia*

[5]*Institute for Materials Research, Tohoku University, Sendai 980-08577, Japan*

[6]*Diamond Light Source Ltd, Harwell Science and Innovation Campus, Didcot OX11 0DE, United Kingdom*

(Dated: May 31, 2025)

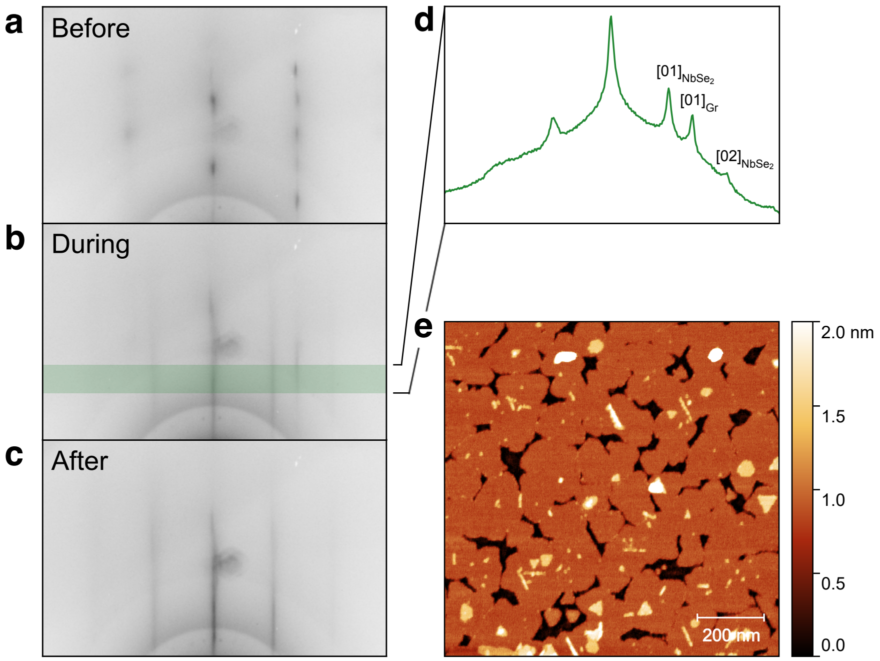


Supplementary Fig. 1. **Materials characterisation.** (a-c) Reflection high-energy electron diffraction measurements of an epitaxial $NbSe_2$/graphite heterostructure: (a) substrate pattern measured before the growth; (b) measurement 65 min into the growth with partial layer coverage, showing clear diffraction streaks from both the graphite and $NbSe_2$ layers; (c) at the end of the growth after 130 min, showing only the film streaks. (d) A line cut through the measured diffraction pattern shown in (b). From this, we extract a bulk-like lattice constant of $3.46 \pm 0.05$ Å of the $NbSe_2$ layer, indicating the absence of any detectable strain being coupled into the epilayer. (e) Corresponding atomic force microscopy measurements, indicating the growth of well-ordered $NbSe_2$ with near-complete coverage of a single monolayer.

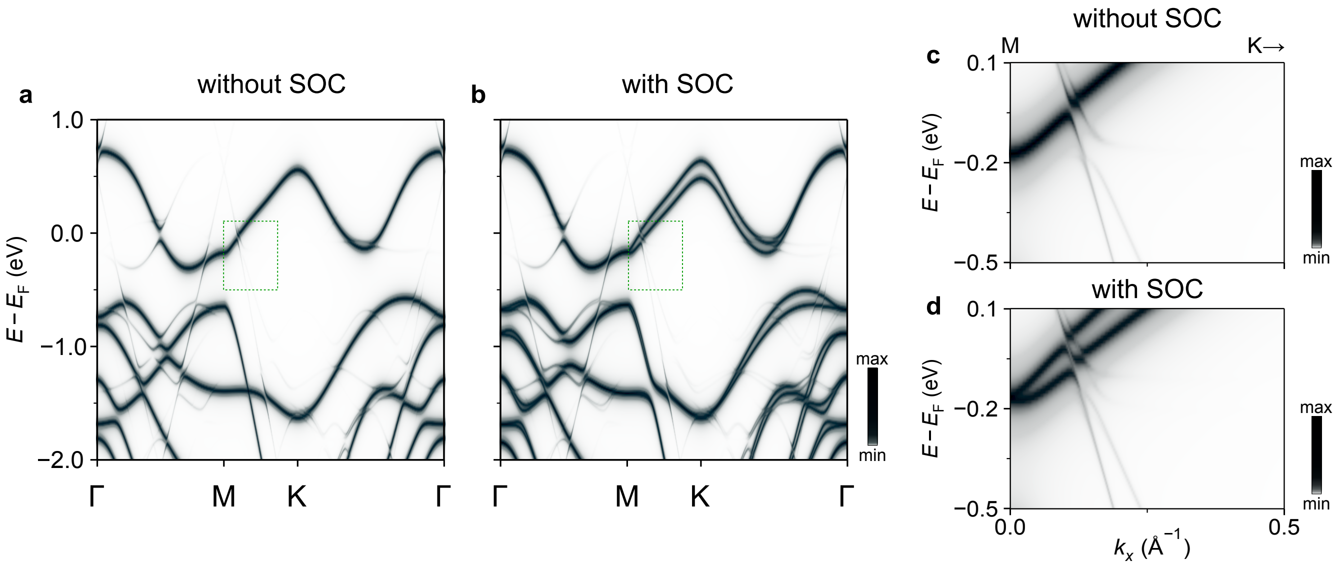


Supplementary Fig. 2. **Influence of spin–orbit coupling on the electronic structure.** Theoretical calculations of the ML-$NbSe_2$/graphene heterostructure bands along Γ-M-K-Γ (in the $NbSe_2$ Brillouin zone) (a) excluding and (b) including spin-orbit coupling. The development of a spin-splitting of the Nb-derived conduction band states is evident in the latter. (c,d) Magnified portion of the band structure along the M-K direction, showing the graphene resonance in the $NbSe_2$ bands (c) without and (d) with spin–orbit coupling.

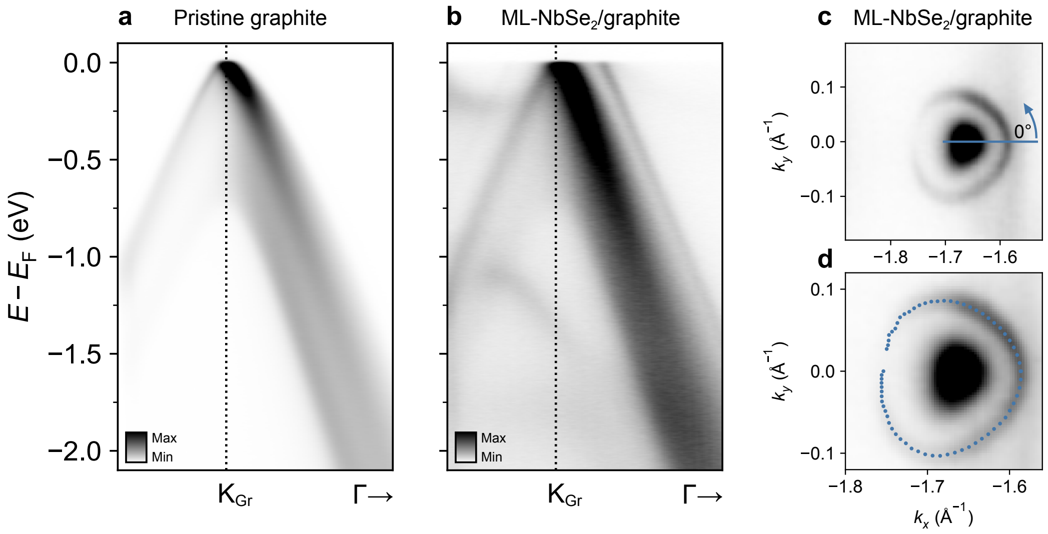


Supplementary Fig. 3. **Interlayer charge transfer.** ARPES measurements ($h\nu = 70$ eV, sum of CL and CR polarisations) of the dispersion along Γ-K in the vicinity of the graphite K point for (a) a pristine graphite sample, and (b) a $NbSe_2$/graphite heterostructure. The latter shows an additional linear band split-off from the $k_z$-dispersive bulk graphite states. This indicates charge transfer from the graphite to the $NbSe_2$ states, hole doping the former. (c) Corresponding Fermi surface measurements in the vicinity of the graphite K point show a well-defined trigonally-warped hole pocket derived from this split-off state. To extract the corresponding Luttinger density, we fit MDCs as a function of the azimuthal angle around the Fermi surface (see arrow). The resulting peak positions are shown in (d).

* These authors contributed equally
† m.saeed.bahramy@manchester.ac.uk
‡ pdk6@st-andrews.ac.uk

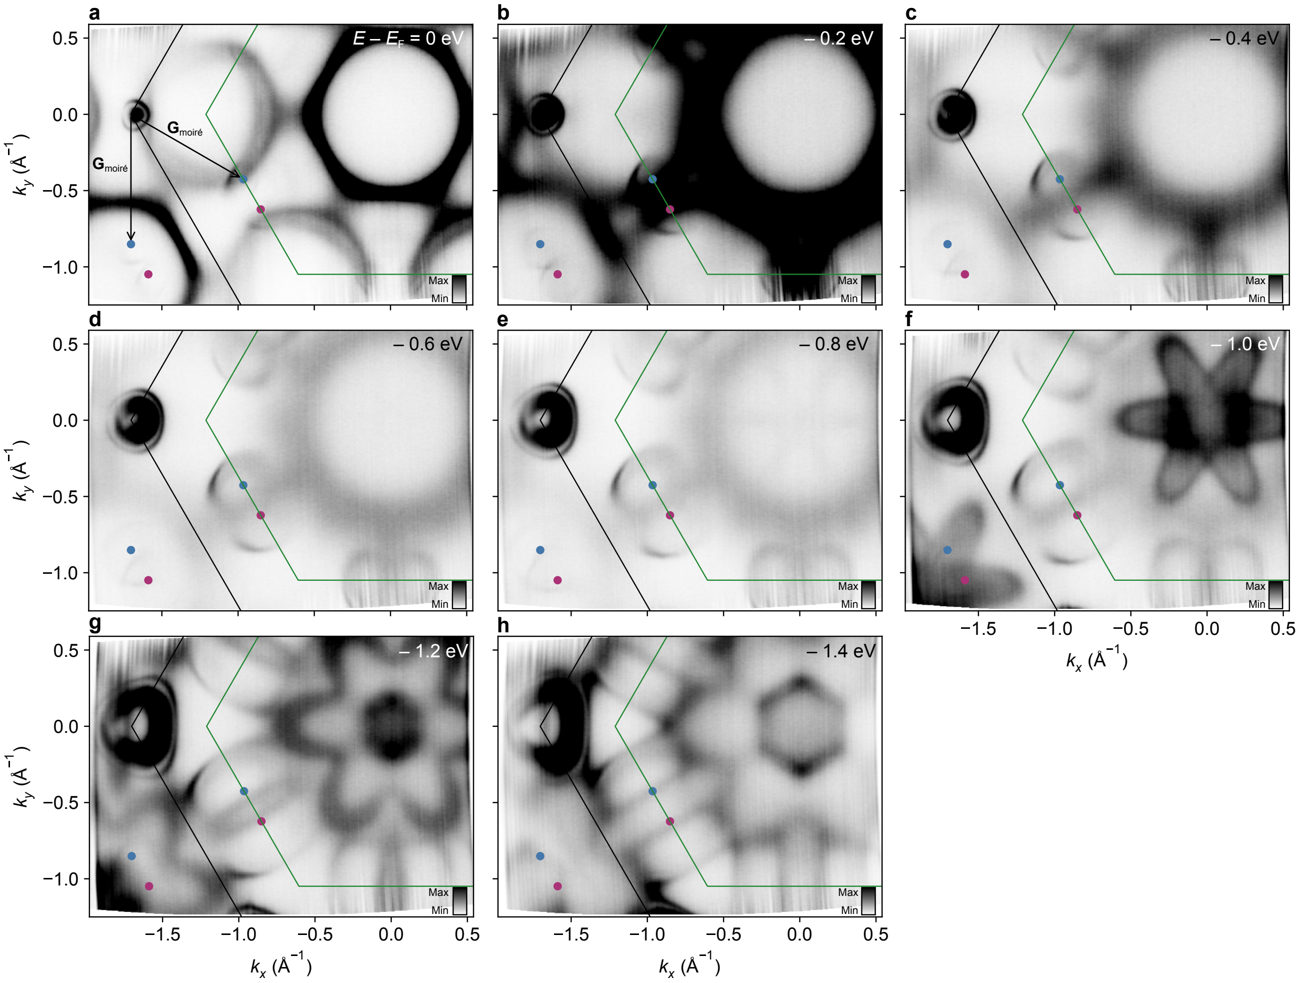


Supplementary Fig. 4. **Constant energy contours.** Measured (a) Fermi surface and (b-h) constant energy contours (see labels for energy). The measurements are the same as shown in Fig. 2(c) of the main text, but are shown here over an extended energy and momentum range and with enhanced contrast.

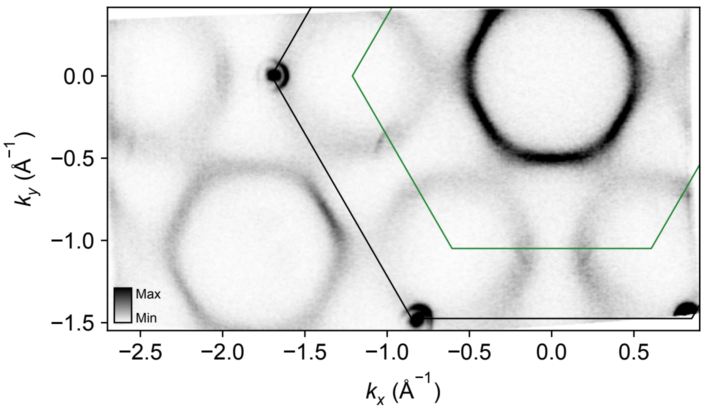


Supplementary Fig. 5. **Additional observation of graphite moiré replicas.** Additional ARPES Fermi surface measurements performed at a photon energy of $h\upsilon = 127$ eV, presented as the sum of spectra measured in CL and CR polarisations, showing clear spectral weight of the graphite moiré replicas where they cross the Nb-derived conduction band states.
